# Supplementary material for: Matrix model approximations of fuzzy scalar field theories and their phase diagrams
Source: arXiv:1510.07496 source file (2016-01-12)
Supplement: Supplementary file 1 [file appendix.tex]

An appendix perhaps?

Effective potential coefficients from (\ref{})
\begin{align}
V_{eff}=&a_{eff} x+\half r_{eff}x^2+h_{eff}x^3+g_{eff}x^4\\
a_{eff}=&-A_1 c_1 \ep+(2  c_1^3-2 c_1 c_2)A_2 \ep^2-3 [A_3 (c_1^5-2 c_1^3 c_2+c_1 c_2^2)-B(3  c_1 c_2^2-\no&
-2 c_1^2 c_3+ c_2 c_3-4 c_1^5+8  c_1^3 c_2)] \ep^3+\ep^4 [A_4 (4 c_1^7-12 c_1^5 c_2+12 c_1^3 c_2^2-4 c_1 c_2^3)+C(200 c_1^7 -600 c_1^5 c_2 +\no&
+480 c_1^3 c_2^2 -80 c_1 c_2^3 +200 c_1^4 c_3 -240 c_1^2 c_2 c_3 +16 c_2^2 c_3 +32 c_1 c_3^2 -40 c_1^3 c_4 +40 c_1 c_2 c_4 -\no&-8 c_3 c_4 )]\\
r_{eff}=&r+A_1 \ep+(-2 A_2 c_1^2+2 A_2 c_2) \ep^2+(3 A_3 c_1^4-12 B c_1^4-6 A_3 c_1^2 c_2+18 B c_1^2 c_2+3 A_3 c_2^2-6 B c_1 c_3) \ep^3+\no&+\ep^4 (-4 A_4 c_1^6+12 A_4 c_1^4 c_2-12 A_4 c_1^2 c_2^2+4 A_4 c_2^3-200 c_1^6 C+480 c_1^4 c_2 C-240 c_1^2 c_2^2 C+32 c_2^3 C-\no&-160 c_1^3 c_3 C+64 c_1 c_2 c_3 C+40 c_1^2 c_4 C-16 c_2 c_4 C)\\
h_{eff}=&(6 B c_1^3-9 B c_1 c_2+3 B c_3) \ep^3+\ep^4 (120 c_1^5 C-240 c_1^3 c_2 C+48 c_1 c_2^2 C+96 c_1^2 c_3 C-24 c_1 c_4 C)\\
g_{eff}=&g+\ep^4 (-40 c_1^4 C+80 c_1^2 c_2 C-16 c_2^2 C-32 c_1 c_3 C+8 c_4 C)
\end{align}
